# Supplementary material for: Ultradense Sphere Packings Derived From Disordered Stealthy Hyperuniform Ground States
Source: arXiv:2504.16924 ancillary file (2025-04-23)
Supplement: Supplementary file 1 [file SM.pdf]

# Supplemental Material: Dense Sphere Packings Derived From Disordered Stealthy Hyperuniform Ground States

Jaeuk Kim

*Princeton Materials Institute, Princeton University, Princeton, NJ 08544, USA*  
*Department of Physics, Princeton University, Princeton, NJ 08544, USA and*  
*Department of Chemistry, Princeton University, Princeton, NJ 08544, USA*

Salvatore Torquato\*

*Department of Chemistry, Princeton University, Princeton, NJ 08544, USA*  
*Department of Physics, Princeton University, Princeton, NJ 08544, USA*  
*Princeton Materials Institute, Princeton University, Princeton, NJ 08544, USA and*  
*Program in Applied and Computational Mathematics,*  
*Princeton University, Princeton, NJ 08544, USA*

## I. SIMULATION PARAMETERS

Table S1 summarizes the simulation parameters employed to generate SHU ground states with or without soft-core repulsions. We consider three different system sizes without soft-core repulsions and two with soft-core repulsions.

TABLE S1. The number of independent configurations  $n_c$  of SHU point patterns with space dimension  $d$ , stealthiness parameter  $\chi$ , and system size  $N$ . For the soft-core cases, we take the maximal target packing fractions listed in Table I.

|         | $\chi \setminus N$ | No soft-core |       |       | Soft-core |      |
|---------|--------------------|--------------|-------|-------|-----------|------|
|         |                    | 400          | 1000  | 2000  | 400       | 1000 |
| $d = 1$ | 0.0025             | 30000        | 10000 | 5000  | 30000     | 5000 |
|         | 0.10               | 30000        | 10000 | 5000  | 30000     | 5000 |
|         | 0.20               | 30000        | 10000 | 5000  | 30000     | 5000 |
|         | 0.30               | 30000        | 10000 | 1500  | 30000     | 5000 |
|         | 0.35               | 30000        | 10000 | 1500  | 30000     | 5000 |
|         | 0.40               | 30000        | 10000 | 1500  | 30000     | 5000 |
|         | 0.45               | 30000        | 10000 | 1500  | 30000     | 5000 |
|         | $\chi \setminus N$ | No soft-core |       |       | Soft-core |      |
|         |                    | 400          | 4000  | 10000 | 400       | 4000 |
| $d = 2$ | 0.0025             | 30000        | 5000  | 1000  | 5000      | 500  |
|         | 0.10               | 30000        | 5000  | 1000  | 5000      | 500  |
|         | 0.20               | 30000        | 5000  | 1000  | 5000      | 500  |
|         | 0.30               | 30000        | 5000  | 1000  | 5000      | 500  |
|         | 0.35               | 30000        | 5000  | 1000  | 5000      | 500  |
|         | 0.40               | 30000        | 5000  | 1000  | 5000      | 500  |
|         | 0.45               | 30000        | 5000  | 1000  | 5000      | 500  |
|         | $\chi \setminus N$ | No soft-core |       |       | Soft-core |      |
|         |                    | 400          | 4000  | 8000  | 400       | 4000 |
| $d = 3$ | 0.0025             | 30000        | 5000  | 1000  | 5000      | 500  |
|         | 0.10               | 30000        | 5000  | 1000  | 5000      | 500  |
|         | 0.20               | 30000        | 5000  | 1000  | 5000      | 500  |
|         | 0.30               | 30000        | 5000  | 1000  | 5000      | 500  |
|         | 0.35               | 30000        | 5000  | 1000  | 5000      | 500  |
|         | 0.40               | 30000        | 5000  | 1000  | 5000      | 500  |
|         | 0.45               | 30000        | 5000  | 1000  | 5000      | 500  |

## II. PLOTS OF $P(r_{\min}; N)$ AND $H_P(r; N)$

Here, we report the plots of minimum-distance distribution  $P(r_{\min}; N)$  and the nearest-neighbor distribution  $H_P(r; N)$  for 1D and 3D SHU ground-state point configurations with  $N$  particles that were briefly described in the main text. For simplicity, we consider three values of  $\chi$  in each dimension:  $\chi = 0.0025, 0.35, 0.45$  for  $d = 1$  and  $\chi = 0.0025, 0.30, 0.45$  for  $d = 3$ .

### A. SHU point patterns without soft-core repulsions

We consider 1D and 3D SHU ground-state point configurations of the standard potential, given in Eq. (2) of the main text. The functional forms of their  $P(r_{\min}; N)$  and  $H_P(r; N)$  vary with dimension  $d$ , but these quantities commonly indicate that the mean value or the variance of  $r_{\min}$  decrease to zero as  $N$  increases. Such a trend is clearly seen when  $\chi$  is below a certain threshold value, i.e.,  $\chi < 1/2$  for  $d = 1$ ,  $\chi \leq 0.35$  for  $d = 2$ , and  $\chi \leq 0.30$  for  $d = 3$ .

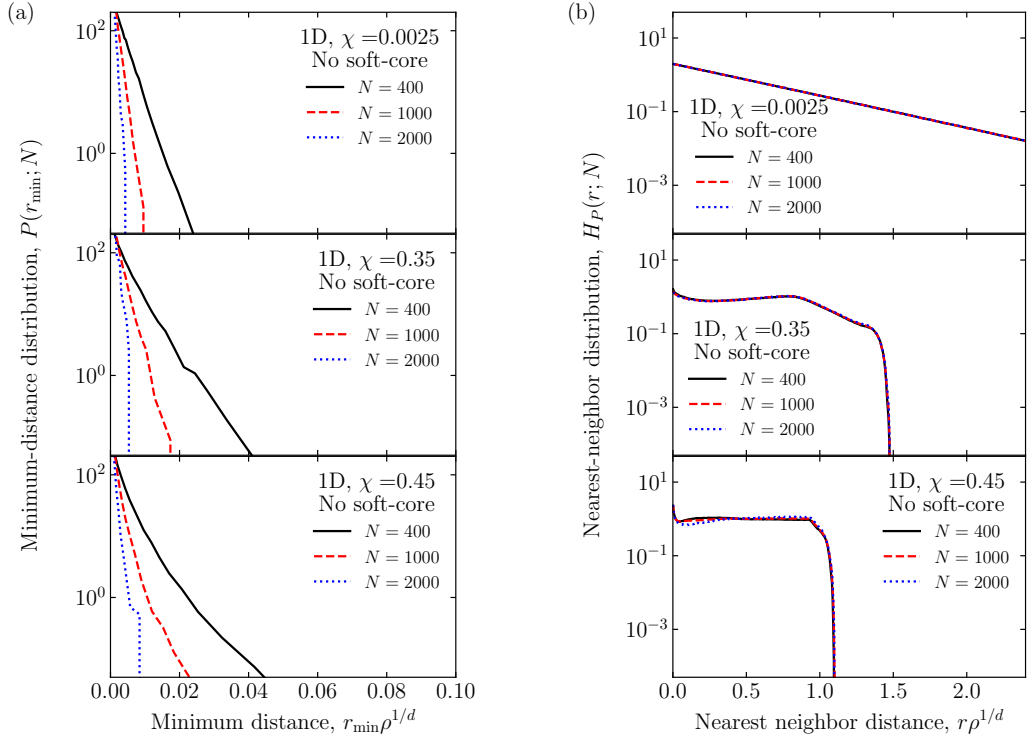

FIG. S1. Semi-log plots of (a) minimum-distance distribution  $P(r_{\min}; N)$  and (b) nearest-neighbor distribution  $H_P(r; N)$  for 1D SHU ground-state point patterns of the standard potential [Eq. (2) of the main text] for  $\chi = 0.0025, 0.35, 0.45$ . Each panel compares the curves with three different system sizes of  $N = 400, 1000, 2000$ .

In one dimension, for any  $\chi < 1/2$ ,  $P(r_{\min}; N)$  exponentially and monotonically decreases with minimum distance  $r_{\min}$ , and its variance also rapidly decreases with  $N$ ; see Fig. S1(a). This observation implies that the majority of 1D SHU point patterns without soft-core repulsions have small values of  $r_{\min}$  (i.e.,  $r_{\min} < 0.05\rho^{-1/2}$ ), and the expectation value of  $r_{\min}$  decreases with  $N$  and eventually vanishes in the thermodynamic limit. We observe that  $H_P(r; N)$  is largely independent of  $N$  for any  $\chi$  in Fig. S1(b), similar to what is seen for  $d = 2$  and  $d = 3$ . However, in contrast to the 2D and 3D cases, we find that  $H_P(r = 0) > 0$ , implying that the 1D SHU point patterns are much more likely to find particles arbitrarily close compared to their higher-dimensional counterparts.

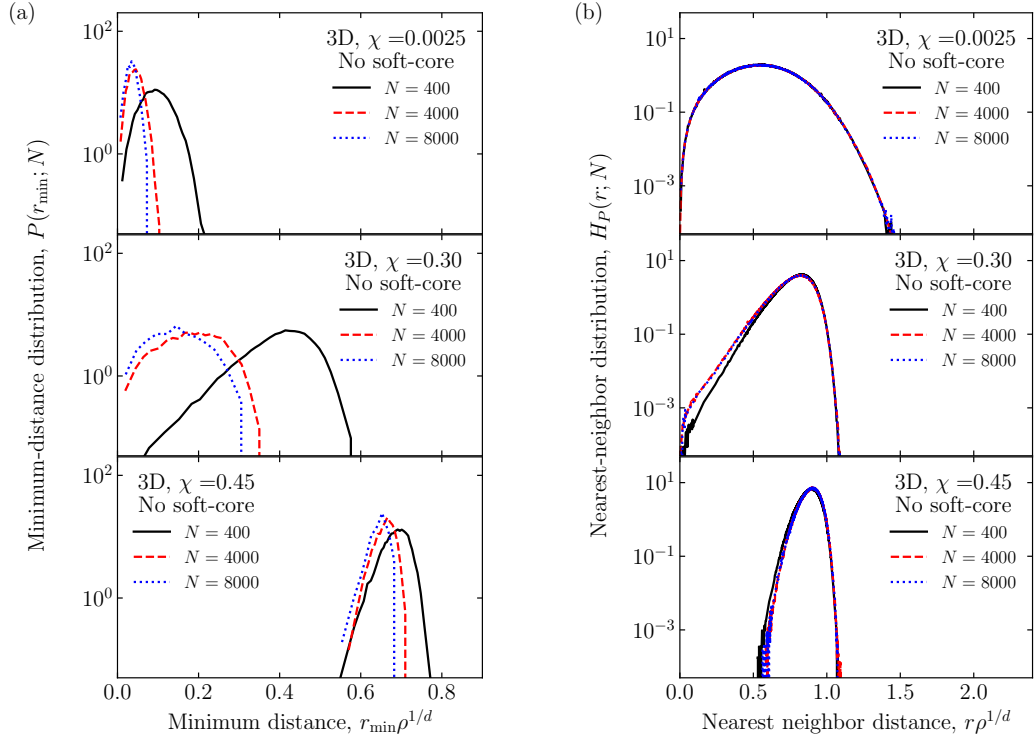

FIG. S2. Semi-log plots of (a) minimum-distance distribution  $P(r_{\min}; N)$  and (b) nearest-neighbor distribution  $H_P(r; N)$  for 3D SHU ground-state point patterns of the standard potential [Eq. (2) of the main text] for  $\chi = 0.0025, 0.30, 0.45$ . Each panel compares the curves with three different system sizes of  $N = 400, 4000, 8000$ .

The local structural characteristics of 3D SHU ground states are virtually identical to those of 2D cases. As shown in Fig. S2(a), for a given  $N$ , the mean value of  $r_{\min}$  monotonically increases with  $\chi$ , but its variance is maximized around a threshold value  $\chi = 0.30$ . By contrast, for a given  $\chi$ , the mean value as well as the variance of  $r_{\min}$  (or  $\phi_{\max}$ ) monotonically decrease as  $N$  increases. The same trend is also observed in two dimensions, but the threshold value is  $\chi = 0.35$  instead of  $\chi = 0.30$ . Figure S2(b) shows that  $H_P(r; N)$  is largely insensitive to  $N$  (except at  $\chi = 0.30$ ), allowing us to practically consider  $H_P(r; N = 8000)$  to be identical to  $H_P(r; \infty) \equiv \lim_{N \rightarrow \infty} H_P(r; N)$ . Thus, using Eq. (9) and simulation data of  $H_P(r; N)$ , we numerically predict that as  $\chi$  increases up to 0.3,  $\phi_{\max}$  is consistent with zero even for the relatively small system sizes of  $N \sim 100$ , as reported in Ref. [1]. Specifically, a 3D SHU ground state with  $N = 100$  and  $\chi = 0.30$  fails to achieve  $\phi_{\max} \gtrsim 0.05$  (or  $r_{\min} \gtrsim 0.457\rho^{1/3}$ ) with a probability of around 50 %, i.e.,

$$\int_0^{0.457/\rho^{1/3}} P(r_{\min}; N = 100) dr_{\min} \approx 1 - \left[ 1 - \int_0^{0.457/\rho^{1/3}} H_P(r; N = 8000) dr \right]^{100/2} \approx 1 - (1 - 0.062)^{100/2} \approx 0.50. \quad (\text{S1})$$

<sup>33</sup> This failure probability increases drastically as  $N$  and  $\phi_{\max}$  increase or  $\chi$  decreases. The analogous analysis for  $\chi \geq 0.4$   
<sup>34</sup> predicts that SHU packings can achieve  $\phi_{\max} \gtrsim 0.10$  with a high probability of around 94% when  $N = 100$ .

### B. SHU point patterns with soft-core repulsions

We consider 1D and 3D SHU ground-state point configurations of the modified potential, given in Eq. (17) of the main text. Two distributions  $P(r_{\min}; N)$  and  $H_P(r; N)$  for the 1D and 3D cases are largely insensitive to  $N$ , similar to their 2D counterparts, shown in Sec. IV B in the main text.

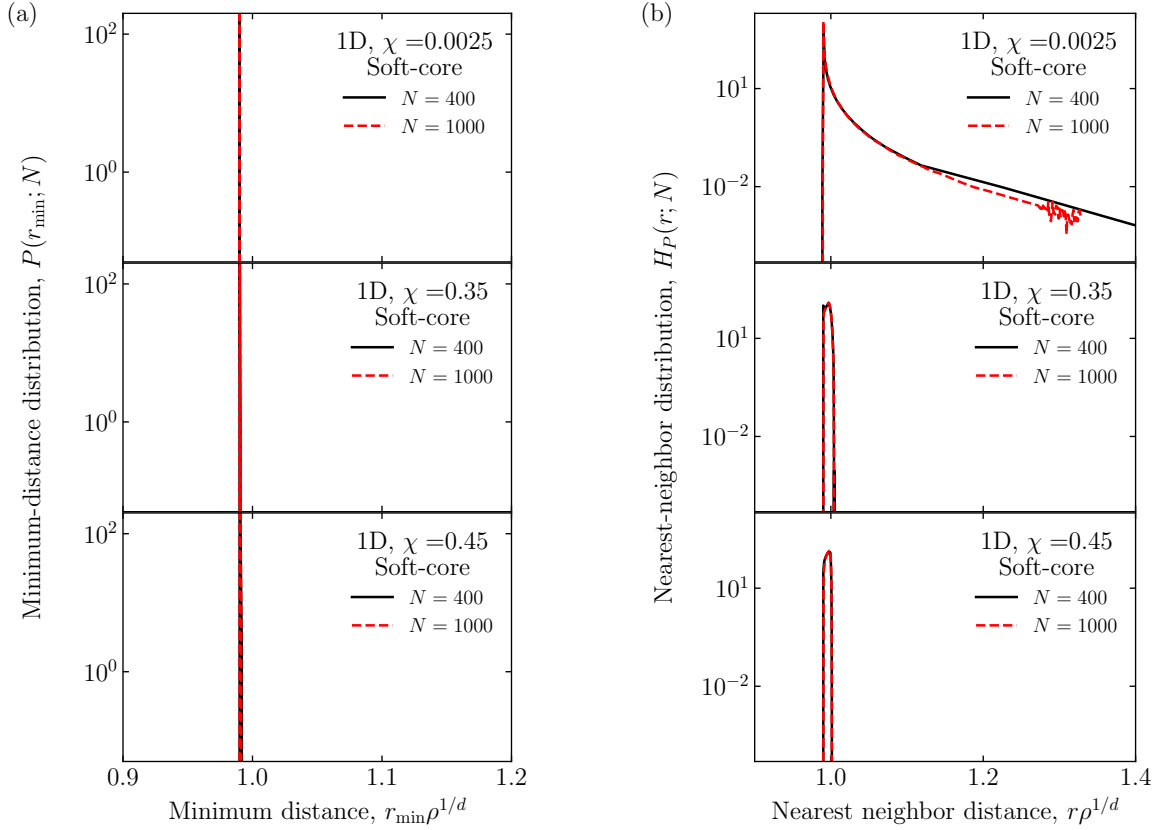

FIG. S3. Semi-log plots of (a) minimum-distance distribution  $P(r_{\min}; N)$  and (b) nearest-neighbor distribution  $H_P(r; N)$  of 1D SHU ground-state point patterns of the modified potential [Eq. (17) of the main text] for  $\chi = 0.0025, 0.35, 0.45$ . Each panel compares the curves with two different system sizes of  $N = 400, 1000$ . Here, we take the target packing fraction  $\phi = 0.99$  for the reason explained in the main text.

In one dimension, for any  $\chi$ , the maximal packing fraction is identical to unity (i.e.,  $\phi_{\max} = 1.0$ ), resulting in perfect integer lattices. Since these perfect integer lattices simply have  $P(r_{\min}; N) = \delta(r - \rho^{-1})$  and  $H_P(r; N) = \delta(r_{\min} - \rho^{-1})$ , we consider 1D ground states with a slightly lower value of target packing fraction  $\phi = \sigma\rho = 0.99$ . As shown in Fig. S3(a),  $P(r_{\min}; N) = \delta(r_{\min} - 0.99\rho^{-1})$  for any  $\chi$ , and thus, there are at least one pair of contacting particles in one ground state. Two particles are taken to be in contact if the pair separation  $r$  obeys the inequality  $r < \sigma + 0.001\rho^{-1/d}$ . By contrast, the range of support in  $H_P(r; N)$  decreases with  $\chi$ ; see Fig. S3(b). At  $\chi = 0.0025$ ,  $H_P(r; N)$  has a broad range of support  $0.99 \leq r\rho \lesssim 1.6$  because the ground states form large domains of dense integer lattices with a lattice spacing of  $0.99\rho^{-1}$ , and the gaps between these domains take on a wide range of values. As  $\chi$  increases up to 0.45, however,  $H_P(r; N)$  converges to a narrow distribution within  $0.99 \leq r\rho \leq 1.01$  because the ground states tend to form smaller domains of such dense integer lattices and resemble the integer lattices of unit lattice spacing.

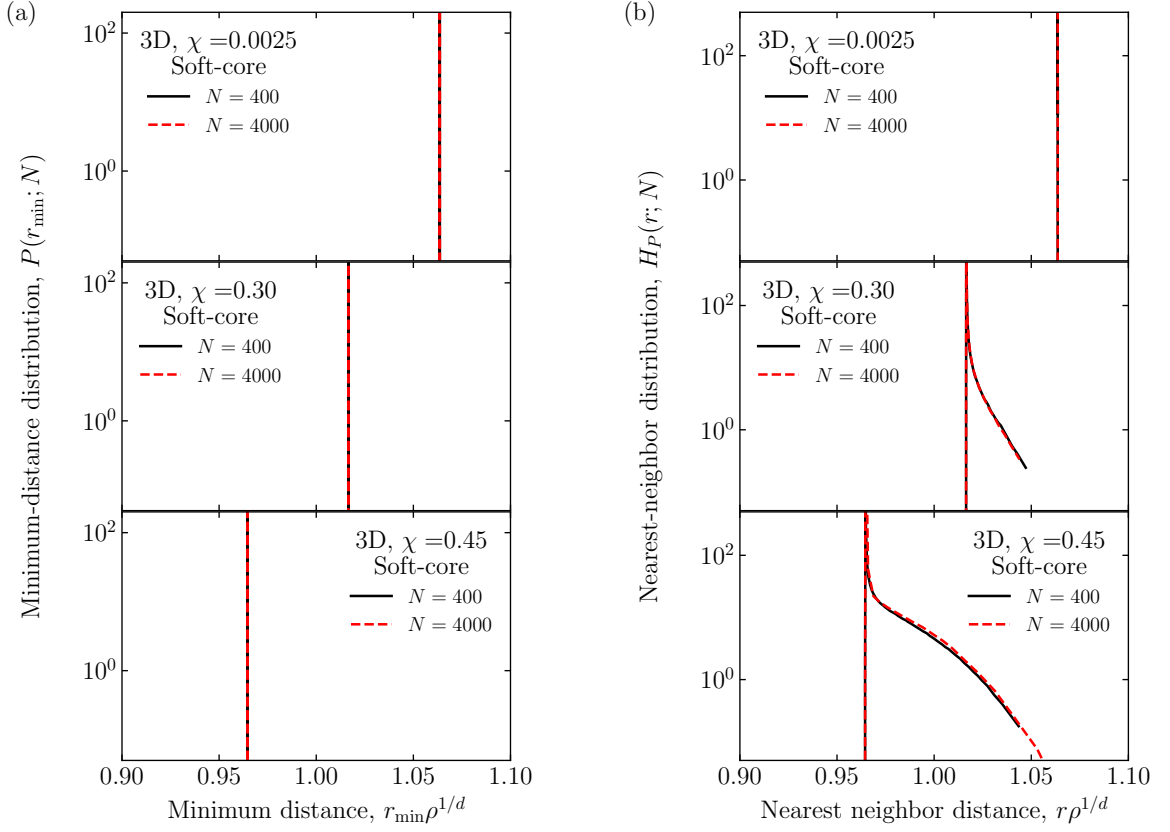

FIG. S4. Semi-log plots of (a) minimum-distance distribution  $P(r_{\min}; N)$  and (b) nearest-neighbor distribution  $H_P(r; N)$  of 3D SHU ground-state point patterns of the modified potential [Eq. (17) of the main text] for  $\chi = 0.0025, 0.30, 0.45$ . Each panel compares the curves with two different system sizes of  $N = 400, 4000$ .

In three dimensions, the functional forms of two distributions  $P(r_{\min}; N)$  and  $H_P(r; N)$  are similar to their 2D counterparts (see Fig. 3 in the main text). In Fig. S4(a), we observe that  $P(r_{\min}; N)$  of 3D ground states behaves like those in dense hard-core systems by construction in that this quantity is a Dirac delta function centered at  $r_{\min} = \sigma$ , implying that each point pattern has particles that are deemed to be in contact. Furthermore, the maximal value of  $\sigma$  or, equivalently, the value of  $\phi_{\max}$  decreases with  $\chi$ . Consistent with these two observations in  $P(r_{\min}; N)$ ,  $H_P(r; N)$  is identically zero for  $r < \sigma$  and possesses a Dirac delta peak at  $r = \sigma$  with  $\sigma$  decreasing with  $\chi$ ; see Fig. S4(b). Similar to the 2D counterparts,  $H_P(r; N)$  has a broader range of support as  $\chi$  increases. However, when  $\chi = 0.0025$ , in contrast to the 2D cases, the function  $H_P(r; N)$  is simply a Dirac delta function because the configurations of these 3D ground states are very close to those of the 3D MRJ state so that each particle has a neighboring particle in contact; see Ref. [2] for detail.

### III. NUMERICAL VERIFICATION OF THE RELATIONSHIP BETWEEN $H_P(r; \infty)$ AND $P(r_{\min}; N)$

Here, we numerically demonstrate the accuracy of the approximate relationship between the nearest-neighbor distribution in the thermodynamic limit  $H_P(r; \infty) \equiv \lim_{N \rightarrow \infty} H_P(r; N)$  and the minimum-distance distribution  $P(r_{\min}; N)$ , given in Eq. (9) of the main text. For this purpose, we solve Eq. (9) for the cumulative distribution function of  $H_P(r; \infty)$  as follows:

$$\int_0^\Delta H_P(r; \infty) dr = 1 - \left[ 1 - \int_0^\Delta P(r_{\min}; N) dr_{\min} \right]^{1/(\gamma N)}, \quad (\text{S2})$$

where  $\gamma = 1/2$  is an empirical correction factor. The validity of Eq. (S2) or, equivalently, Eq. (9) of the main text can be easily confirmed by showing whether the cumulative distribution functions of  $H_P(r; \infty)$  estimated from  $P(r_{\min}; N)$  with different  $N$  collapse on a single curve. We immediately see that the cumulative distribution functions of  $H_P(r; \infty)$  from the  $P(r_{\min}; N)$  collapse on a single curve in Fig. S5, meaning that Eq. (9) is accurate, except for  $\chi = 0.35$ . We also confirm that Eq. (9) is accurate for all  $\chi$  values except for the following cases:  $\chi = 0.30, 0.35$  in two dimensions and  $\chi = 0.30$  in three dimensions.

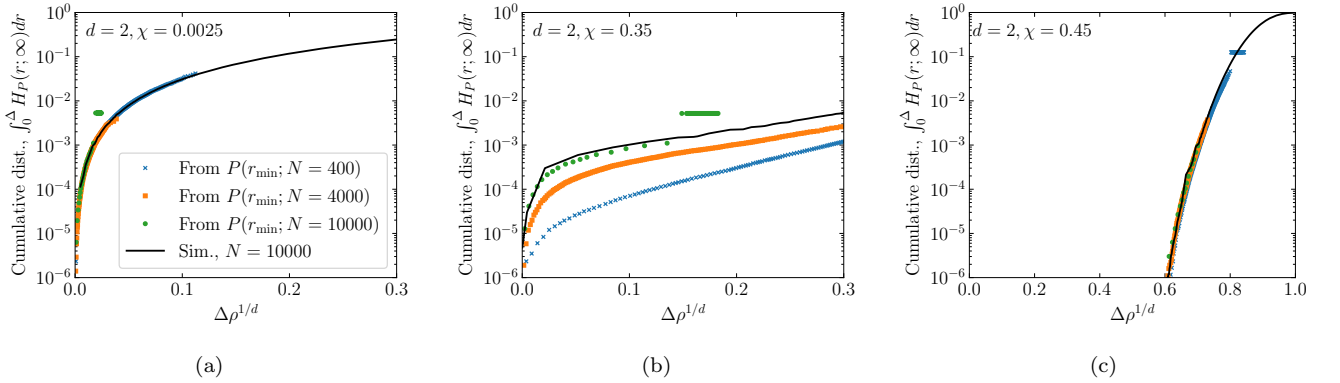

FIG. S5. Semi-log plot of the cumulative distribution functions of  $H_P(r; \infty)$  as functions of dimensionless distance  $\Delta \rho^{1/d}$  for 2D SHU ground-state point patterns without soft-core repulsions with three values of (a)  $\chi = 0.0025$ , (b)  $\chi = 0.35$ , and (c)  $\chi = 0.45$ . The cumulative distributions are estimated from the minimum-distance distributions  $P(r_{\min}; N)$  with  $N = 400, 4000, 10000$  using Eq. (S2) or obtained from direct simulations with  $N = 10000$ .

TABLE S2. Fractions of 2D SHU ground states generated without soft-core repulsions that fail to achieve packing fraction  $\phi$  for a range of  $\chi$  and  $N$ . All fractions are presented as percentages, meaning that 0.0 [%] is always achievable, whereas 100.0 [%] is always failing.

| $\phi$ | $\chi = 0.0025$ |       |       | $\chi = 0.10$ |       |       | $\chi = 0.20$ |       |       | $\chi = 0.30$ |       |       | $\chi = 0.35$ |       |       | $\chi = 0.40$ |       |       | $\chi = 0.45$ |      |       |
|--------|-----------------|-------|-------|---------------|-------|-------|---------------|-------|-------|---------------|-------|-------|---------------|-------|-------|---------------|-------|-------|---------------|------|-------|
|        | 400             | 4000  | 10000 | 400           | 4000  | 10000 | 400           | 4000  | 10000 | 400           | 4000  | 10000 | 400           | 4000  | 10000 | 400           | 4000  | 10000 | 400           | 4000 | 10000 |
| 0.0001 | 7.8             | 53.9  | 89.0  | 8.8           | 65.2  | 93.7  | 12.1          | 91.2  | 99.8  | 5.1           | 85.5  | 100.0 | 0.1           | 5.1   | 31.2  | 0.0           | 0.0   | 0.0   | 0.0           | 0.0  | 0.0   |
| 0.0010 | 55.1            | 99.8  | 100.0 | 55.5          | 100.0 | 100.0 | 62.1          | 100.0 | 100.0 | 27.0          | 100.0 | 100.0 | 0.3           | 20.7  | 78.1  | 0.0           | 0.0   | 0.0   | 0.0           | 0.0  | 0.0   |
| 0.0100 | 100.0           | 100.0 | 100.0 | 99.9          | 100.0 | 100.0 | 99.8          | 100.0 | 100.0 | 78.7          | 100.0 | 100.0 | 1.7           | 60.5  | 98.4  | 0.0           | 0.0   | 0.0   | 0.0           | 0.0  | 0.0   |
| 0.1000 | 100.0           | 100.0 | 100.0 | 100.0         | 100.0 | 100.0 | 100.0         | 100.0 | 100.0 | 100.0         | 100.0 | 100.0 | 40.2          | 100.0 | 100.0 | 0.0           | 0.0   | 0.3   | 0.0           | 0.0  | 0.0   |
| 0.2000 | 100.0           | 100.0 | 100.0 | 100.0         | 100.0 | 100.0 | 100.0         | 100.0 | 100.0 | 100.0         | 100.0 | 100.0 | 96.7          | 100.0 | 100.0 | 1.1           | 19.9  | 50.0  | 0.0           | 0.0  | 0.0   |
| 0.3000 | 100.0           | 100.0 | 100.0 | 100.0         | 100.0 | 100.0 | 100.0         | 100.0 | 100.0 | 100.0         | 100.0 | 100.0 | 100.0         | 100.0 | 100.0 | 46.1          | 100.0 | 100.0 | 0.0           | 0.4  | 1.5   |
| 0.4000 | 100.0           | 100.0 | 100.0 | 100.0         | 100.0 | 100.0 | 100.0         | 100.0 | 100.0 | 100.0         | 100.0 | 100.0 | 100.0         | 100.0 | 100.0 | 99.9          | 100.0 | 100.0 | 24.0          | 96.5 | 100.0 |

TABLE S3. Fractions of 3D SHU ground states generated without soft-core repulsions that fail to achieve packing fraction  $\phi$  for a range of  $\chi$  and  $N$ . All fractions are presented as percentages, meaning that 0.0 [%] is always achievable, whereas 100.0 [%] is always failing.

[illegible]

## V. PROBABILISTIC UPPER BOUND ON $\phi_{\max}$ FOR SHU GROUND-STATE CONFIGURATIONS WITHOUT SOFT-CORE REPULSIONS.

Here, we provide details of generating the contour plots of the ratio  $p_{\text{fail}}/N$  as functions of  $\phi_{\max}$  and  $\chi$ , shown in Fig. 4 of the main text. At each value of  $\chi$ , we obtain a curve of  $p_{\text{fail}}/N$  as a function of  $\phi_{\max} = \rho v_1(\Delta/2)$  by computing the cumulative distribution function of  $H_P(r; \infty)$  in the thermodynamic limit, i.e.,  $\int_0^\Delta H_P(x; \infty) dx$ ; see Eq. (22) in the main text. When the ratio  $p_{\text{fail}}/N \geq 10^{-4}$ , we directly take the simulation data of the cumulative distributions. By contrast, when the ratio is smaller than  $10^{-4}$ , we evaluate the ratio from the converse Weibull distribution with three fitting parameters  $a'(\chi, d)$ ,  $b'(\chi, d)$ , and  $c'(\chi, d)$  that are dependent on  $d$  and  $\chi$ :

$$\int_0^r H_P(x; \infty) dx \approx 1 - \exp\left\{-[(r - a')/b']^{c'}\right\}, \quad a' < r, \quad (\text{S3})$$

where  $a'$  is a position parameter,  $b' > 0$  is a scale parameter, and  $c' > 0$  is a shape parameter. This conjecture is based on *the asymptotic law of minima* [3, 4], as articulated in Sec. V A. However, since Eq. (S3) is inaccurate for probabilities greater than 0.01, and we need the fitting only in the low-probability regime, we use the following simplified fit function for probabilities between  $10^{-6}$  and  $10^{-3}$ :

$$\int_0^r H_P(x; \infty) dx \approx \left(\frac{r - a'}{b'}\right)^{c'}. \quad (\text{S4})$$

We tabulate the resulting parameters for 2D and 3D cases in Table S4. We note that  $|a'(\chi, d)| < 10^{-30}$  for any  $\chi$  and  $d$ .

TABLE S4. Parameters  $a'(\chi, d)$ ,  $b'(\chi, d)$ , and  $c'(\chi, d)$  in the Weibull-distribution approximation (S3) to model the nearest-neighbor distribution function  $H_P(r; \infty)$  of 2D and 3D SHU ground-state point patterns without soft-core repulsions in the thermodynamic limit, i.e.,  $N \rightarrow \infty$ . The parameters are estimated by fitting the cumulative distribution functions of  $H_P(r; \infty)$  with Eq. (S4) within the range where the probability values lie between  $10^{-6}$  and  $10^{-3}$ . We utilize the simulation data from the largest systems:  $N = 10000$  for  $d = 2$  and  $N = 8000$  for  $d = 3$ .

| $\chi$ | $d = 2$       |               |               | $d = 3$       |               |               |
|--------|---------------|---------------|---------------|---------------|---------------|---------------|
|        | $a'(\chi, d)$ | $b'(\chi, d)$ | $c'(\chi, d)$ | $a'(\chi, d)$ | $b'(\chi, d)$ | $c'(\chi, d)$ |
| 0.0025 | 0.000         | 0.601         | 1.946         | 0.000         | 0.726         | 2.769         |
| 0.10   | 0.000         | 0.673         | 1.831         | 0.000         | 0.884         | 2.690         |
| 0.20   | 0.000         | 0.592         | 1.609         | 0.000         | 1.376         | 2.376         |
| 0.30   | 0.000         | 0.861         | 1.468         | 0.000         | 11.596        | 1.991         |
| 0.35   | 0.000         | 22.040        | 1.293         | 0.000         | 1.032         | 8.731         |
| 0.40   | 0.000         | 0.826         | 17.660        | 0.000         | 0.854         | 19.007        |
| 0.45   | 0.000         | 0.815         | 43.964        | 0.000         | 0.840         | 32.727        |

77 In 2D cases without soft-core repulsions, the simulation data of  $\int_0^r H_P(x; \infty) dx$  show excellent agreement with  
 78 the fitted curves from Eq. (S3) and Table S4 for all values of  $\chi$ . This can be seen in the upper panels of Fig.  
 79 S6. Additionally, substituting the fitted curve to Eq. (9) accurately estimates the minimum-distance distribution  
 80  $P(r_{\min}; N)$  as shown in the lower panels of Fig. S6. Similarly, for the 3D cases, the simulation data and the fitted  
 81 curves demonstrate excellent agreement for all  $\chi$ , except for  $\chi = 0.35$ , as illustrated in Fig. S7.

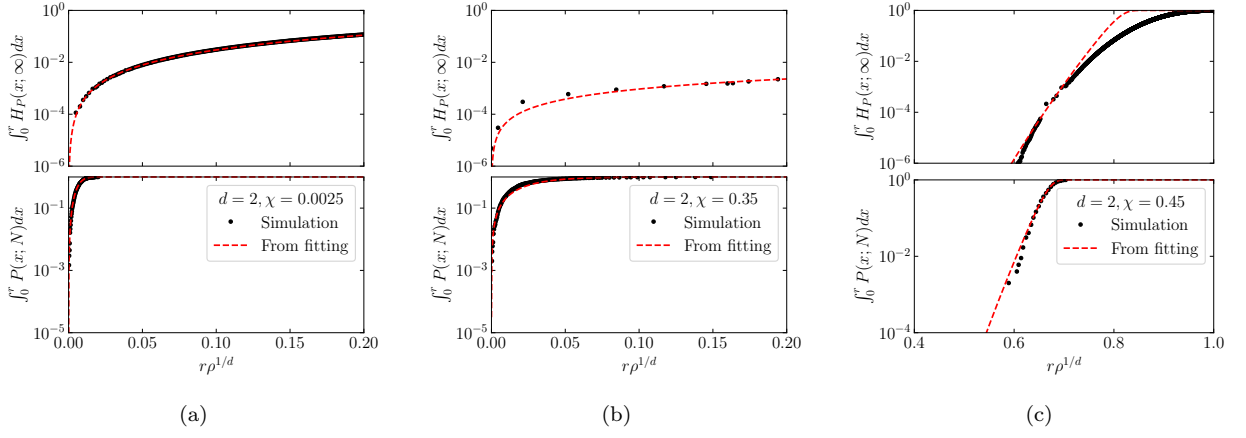

FIG. S6. Comparisons of simulation data and their fitted curves for the cumulative distribution functions of (Upper)  $H_P(x; \infty)$  and (Lower)  $P(x; N)$  from 2D SHU ground states without soft-core repulsions. Three values of  $\chi$  are considered: (a)  $\chi = 0.0025$ , (b)  $\chi = 0.35$ , and (c)  $\chi = 0.45$ . The simulation data are from the largest systems with  $N = 10000$ . All panels are drawn in a semi-log scale. The fit curves on the upper panels are evaluated from Eq. (S3) and the parameters in Table S4. These curves are used to evaluate the curves on the lower panels by using Eq. (9) in the main text.

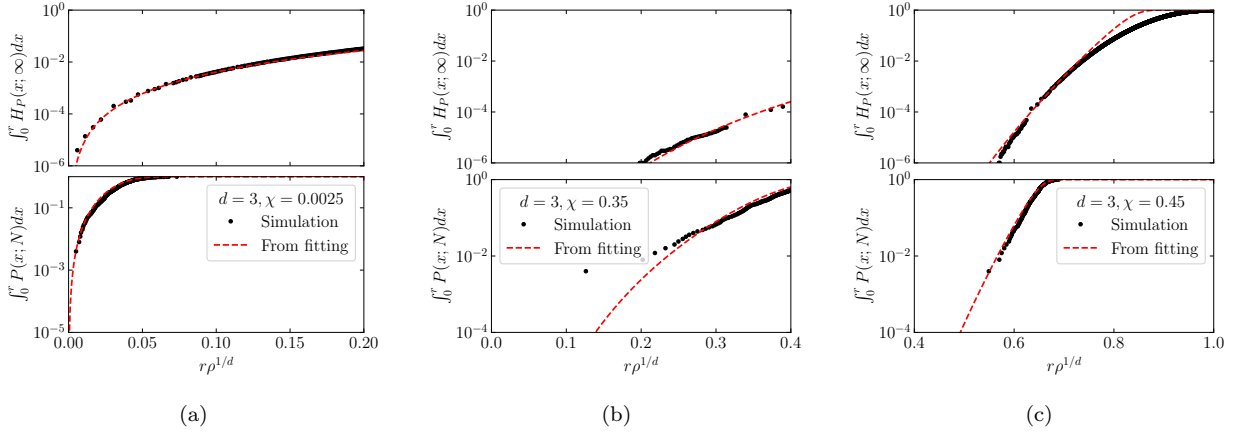

FIG. S7. Comparisons of simulation data and their fitted curves for the cumulative distribution functions of (Upper)  $H_P(x; \infty)$  and (Lower)  $P(x; N)$  from 3D SHU ground states without soft-core repulsions. Three values of  $\chi$  are considered: (a)  $\chi = 0.0025$ , (b)  $\chi = 0.35$ , and (c)  $\chi = 0.45$ . The simulation data are from the largest systems with  $N = 8000$ . All panels are drawn in a semi-log scale. The fit curves on the upper panels are evaluated from Eq. (S3) and the parameters in Table S4. These curves are used to evaluate the curves on the lower panels by using Eq. (9) in the main text.

### A. Asymptotic Law of Minima

Here, we explain our rationale on Eq. (S3). We first state the asymptotic law of minima, also known as the Fisher-Tippett theorem [3, 4]:

**Theorem 1** Let  $X_1, \dots, X_n$  be a sample of independent and identically distributed random variables and  $\tilde{M}_n = \min\{X_1, \dots, X_n\}$ . If norming sequences  $\{a_n\}$  and  $\{b_n > 0\}$  exist such that

$$\lim_{n \rightarrow \infty} \text{Probability} \left\{ \frac{\tilde{M}_n - a_n}{b_n} \leq z \right\} = G(z), \quad z \in \mathbb{R}, \quad (\text{S5})$$

where  $G(z)$  is a non-degenerate distribution, then  $G(z)$  belongs to one of the following three types of limit (or asymptotic) distributions of minima:

1. (Converse) Weibull

$$G(z) = \begin{cases} 0, & z < a', \\ 1 - \exp \left\{ -[(x - a')/b']^{c'} \right\}, & z \geq a'; \end{cases} \quad (\text{S6})$$

2. (Converse) Gumbel

$$G(z) = 1 - \exp \left\{ -\exp \left( \frac{z - a'}{b'} \right) \right\}, \quad -\infty < z < \infty; \quad (\text{S7})$$

3. (Converse) Fréchet

$$G(z) = \begin{cases} 1 - \exp \left\{ -[-(z - a')/b']^{-c'} \right\}, & z \leq a' \\ 1, & z > a'. \end{cases} \quad (\text{S8})$$

Here,  $a' \in \mathbb{R}$  is a position parameter,  $b' > 0$  is a scale parameter, and  $c' > 0$  is a shape parameter.

Denoting the cumulative distribution function of a random variable  $X_i$  by  $F(z)$ , we note that the asymptotic distribution is determined by the ‘left tail’ of  $F(z)$ . If the support of  $F(z)$  is bounded from below so that its probabilities are low on the left tail, the limit distribution becomes the Weibull distribution. Examples of such  $F(z)$  include the uniform, exponential, gamma, and Pareto distributions. If  $F(z)$  has an exponentially decaying left tail (e.g., Gaussian and lognormal distributions),  $G(z)$  becomes the Gumbel distribution. By contrast,  $G(z)$  becomes the Fréchet distribution if  $F(z)$  has a heavy left tail with a power-law decay (e.g., Cauchy distribution) and if the support of  $F(z)$  is not bounded from below.

We note that the asymptotic law of minima is approximately applicable to the nearest-neighbor distribution. Specifically, for one particle of a point pattern with  $N$  particles, its nearest-neighbor distance is the ‘minimum’ of  $N - 1$  pair distances, each of which is obviously nonnegative (i.e., bounded from below by 0). Therefore, as we explained above, the cumulative distribution of  $H_P(r; \infty)$  follows the Weibull distribution among Eqs. (S6)-(S8) in the thermodynamic limit. We can easily confirm this conjecture in the case of the Poisson point patterns. For the Poisson point patterns with number density  $\rho$  in  $d$  dimensions, the cumulative distribution function of  $H_P(r; \infty)$  is known analytically [5]:

$$1 - E_P(r) = \int_0^r H_P(x; \infty) dx = 1 - \exp[-\rho v_1(r)], \quad r \geq 0, \quad (\text{S9})$$

which is the Weibull distribution with  $a' = 0, b' = [\rho v_1(1)]^{-1/d}, c' = d$ . Here, the particle exclusion probability  $E_P(r)$  is the probability of finding a spherical region of radius  $r$  that is centered at a particle but empty of other particle centers. We note that Eq. (S3) is no longer valid if there are strong correlations in pair distances, such as dense packings of hard spheres.

## VI. MEAN CONTACT NUMBER

Here, we present the mean contact number per particle  $Z(r = \sigma^+)$  for 2D and 3D ultradense SHU packings with different choices of  $\sigma^+ = \sigma + \epsilon$ ; see Fig. S8. Note that the value of  $Z(r = \sigma^+)$  monotonically increases with the tolerance  $\epsilon$ . In the main text, we solely take  $\epsilon = 0.001\rho^{-1/d}$  for simplicity.

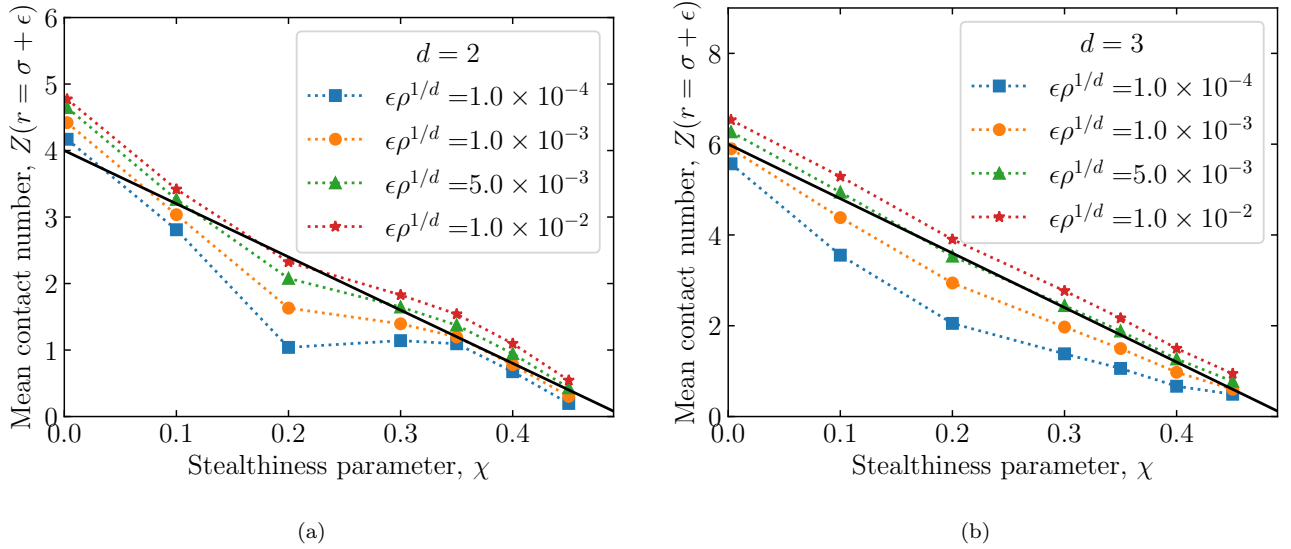

FIG. S8. Mean contact numbers  $Z(r = \sigma + \epsilon)$  as functions of stealthiness parameter  $\chi$  for ultradense SHU packings in (a)  $d = 2$  and (b)  $d = 3$ . Each data point is computed by integrating  $g_2(r)$  up to  $r = \sigma + \epsilon$ . We consider ground states with  $N = 4000$ .

## VII. PAIR STATISTICS OF 1D SYSTEMS

Here, we report the structure factor  $S(k)$  and the pair correlation function  $g_2(r)$  of 1D SHU point patterns with and without soft-core repulsions for the smallest  $\chi (= 0.0025)$  and the largest  $\chi (= 0.45)$ . For the reason that we described in Sec. II B, we consider 1D ultradense ground states with  $\phi = \sigma\rho = 0.99$  instead of  $\phi = 1.00$ .

We begin by considering 1D SHU ground states for the smallest  $\chi (= 0.0025)$  shown in Fig. S9(a,d). Without soft-core repulsion, 1D SHU ground state is almost like ideal gas, except that  $S(k = 0) = 0$ . When soft-core repulsions are turned on,  $g_2(r)$  exhibits asymmetric peaks with the left sides abruptly emerging at  $r\rho = 0.99n$  for  $n = 1, 2, \dots$  and the right sides decaying relatively slowly. Furthermore,  $S(k)$  has broadened Bragg peaks at  $k\rho^{-1} = 2\pi/0.99$  for  $n = 1, 2, \dots$ ; see the cyan lines in the lower panel of Fig. S9(a). These two observations imply that the 1D ultradense SHU ground state becomes a polycrystalline integer lattice whose lattice spacing is  $\sigma = 0.99\rho^{-1}$ .

As  $\chi$  increases to 0.35, the 1D SHU ground state without soft-core repulsion shows a drastic change in its  $S(k)$ : it becomes zero around  $k = \pi\rho$ , which is not explicitly constrained to be zero in the collective-coordinate optimization procedure; see Fig. S9(b). By contrast,  $g_2(r)$  slightly suppressed around the origin. The ultradense SHU ground state, however, become an integer lattice with unit lattice spacing, indicated by both  $S(k)$  and  $g_2(r)$ .

Figure S9(c,f) shows pair statistics for 1D SHU ground states for the highest  $\chi$ . When there are no soft-core repulsions,  $g_2(r)$  has broadened peaks centered at  $r\rho = 2, 4, \dots$ , and  $S(k)$  also have broadened and decaying peaks at  $k\rho^{-1} = \pi, 2\pi, \dots$ . Both observations indicate that the ground states are superpositions of two distinct imperfect integer lattices with lattice spacing  $2\rho^{-1}$ . By contrast, when soft-core repulsions are turned on,  $g_2(r)$  exhibits symmetric peaks at  $r\rho = n$  for  $n = 1, 2, \dots$ , and  $S(k)$  also have symmetric and sharp peaks at  $k\rho^{-1} = 2\pi, 4\pi, \dots$ . Therefore, the corresponding ground states are configurationally very close to perfect integer lattices of lattice spacing  $\rho^{-1}$ .

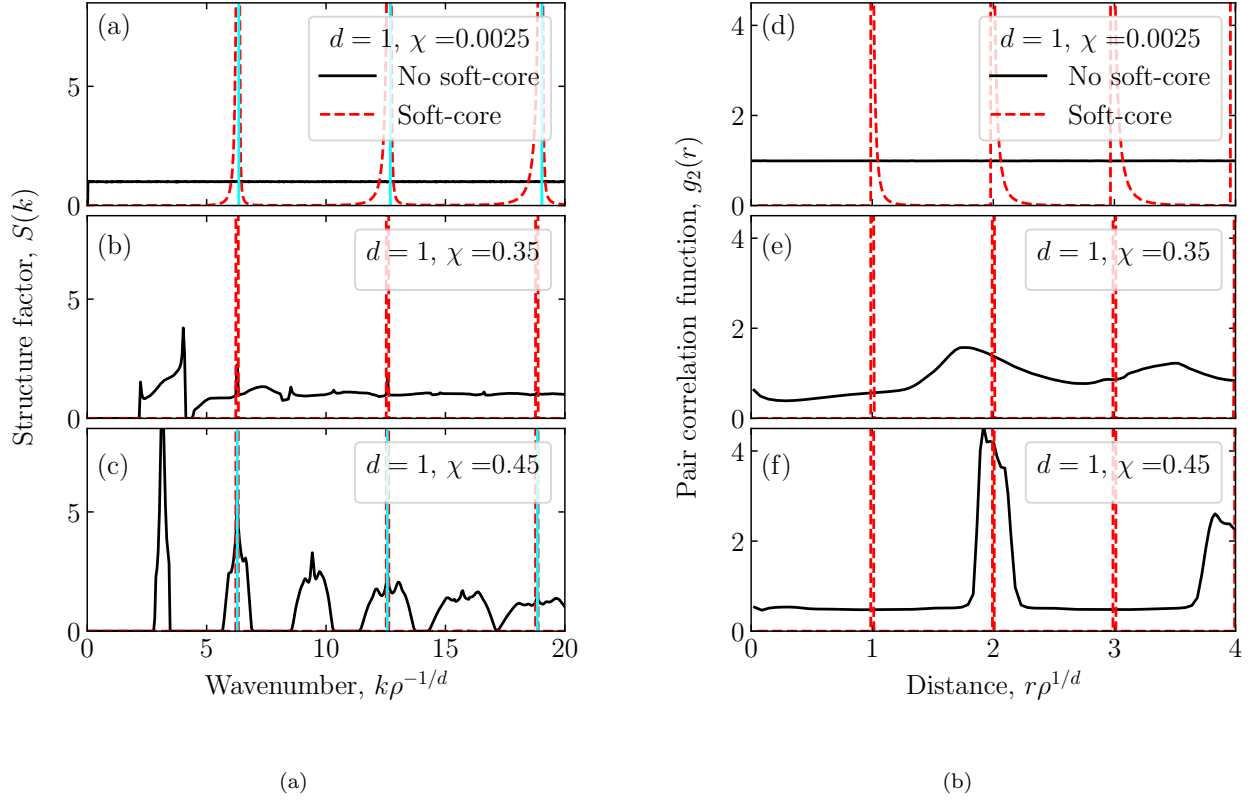

FIG. S9. Pair statistics of 1D SHU ground-state point patterns of  $N = 400$  with and without soft-core repulsions at  $\chi = 0.0025, 0.35$ , and  $0.45$ : (a-c) Structure factor  $S(k)$  and (e-f) pair correlation function  $g_2(r)$ . In the cases with the soft-core repulsion, we take  $\phi = 0.99$ . In (a) and (c), the cyan vertical lines for  $S(k)$  depict  $k\rho^{-1/d} = 2\pi n/0.99$  and  $k\rho^{-1/d} = 2\pi n$ , respectively, where  $n = 1, 2, \dots$ .

- [1] G. Zhang, F.H. Stillinger, and S. Torquato, "Transport, geometrical, and topological properties of stealthy disordered hyperuniform two-phase systems," J. Chem. Phys. **145**, 244109 (2016).
- [2] S. Torquato and J. Kim, "Existence of nonequilibrium glasses in the degenerate stealthy hyperuniform ground-state manifold," preprint (2025).
- [3] G. Salvadori, ed., *Extremes in nature: an approach using copulas*, Water science and technology library No. 56 (Springer, Dordrecht, 2007).
- [4] M. I. Gomes and A. Guillou, "Extreme value theory and statistics of univariate extremes: A review," Int. Stat. Rev. **83**, 263–292 (2015).
- [5] S. Torquato, *Random Heterogeneous Materials: Microstructure and Macroscopic Properties*, Interdisciplinary Applied Mathematics No. 16 (Springer Science & Business Media, New York, 2002).
